# Supplementary material for: Quantum Simulation of non-Abelian Lattice Gauge Theories: a variational approach to $\mathbb{D}_8$
Source: arXiv:2501.17863 source file (2025-01-29)
Supplement: Supplementary file 1 [file appendixB.tex]

Here, we provide the necessary material for the calculation of the exact spectra in various analyses of the pseudo-2D model.

\begin{figure}[h]
    \centering
\[ H = 
\scalebox{0.75}{\begin{bmatrix}
  2M & 0 & 0 &  0 & 0 & 0 & 0 & -J \sqrt{2} & 0 & 0\\
  0 & 2M & 0 & 0 & 0 & 0 & 0 & 0 & 0 & -J \sqrt{2} \\
  0 & 0 & 2M & 0 & 0 & 0 & 0 & 0 & -J \sqrt{2} & 0\\
  0 & 0 & 0  & -2M & 0 & 0 & 0 & -J \sqrt{2} & -J \sqrt{2} & -J \sqrt{2}\\
  0 & 0 & 0  & 0   & M + 2\lambda_E& 0 & 0 & -J & 0 & -J\\
  0 & 0 & 0  &   0 &  0  &  M + 2\lambda_E & 0 & -J & -J & 0\\
  0 & 0 & 0  &  0  &  0  &  0  &   M + 2\lambda_E & 0 & -J & -J\\
  -J \sqrt{2} & 0 & 0  &  -J \sqrt{2}  &  -J  &  -J  &  0  &  \lambda_E & 0 & 0\\
  0 & 0 & -J \sqrt{2}  & -J \sqrt{2}   &  0 & -J  &  -J  &  0  & \lambda_E & 0\\
  0 & -J \sqrt{2} & 0  &  -J \sqrt{2}  &  -J  & 0   & -J   & 0   &  0  &   \lambda_E
\end{bmatrix}}
\]    \caption{Original Hamitonian evaluated over the ten gauge invariant states.}
  \label{Matrix_with_matter}
\end{figure}
\begin{figure}
    \centering
\[ H^{(2)} = \scalebox{0.7}{ 
\begin{bmatrix}
  2M & 0 & 0 &  0 & 0 & 0 & 0 & -iJ \sqrt{2} & 0 & 0\\
  0 & 2M & 0 & 0 & 0 & 0 & 0 & 0 & 0 & iJ \sqrt{2} \\
  0 & 0 & 2M & 0 & 0 & 0 & 0 & 0 & iJ \sqrt{2} & 0\\
  0 & 0 & 0  & -2M & 0 & 0 & 0 & -iJ \sqrt{2} & iJ \sqrt{2} & iJ \sqrt{2}\\
  0 & 0 & 0  & 0   & M + 2\lambda_E& 0 & 0 & iJ & 0 & -iJ\\
  0 & 0 & 0  &   0 &  0  &  M + 2\lambda_E & 0 & iJ & -iJ & 0\\
  0 & 0 & 0  &  0  &  0  &  0  &   M + 2\lambda_E & 0 & iJ & iJ\\
  iJ \sqrt{2} & 0 & 0  &  iJ \sqrt{2}  &  -iJ  &  -iJ  &  0  &  \lambda_E & 0 & 0\\
  0 & 0 & -iJ \sqrt{2}  & -iJ \sqrt{2}   &  0 & iJ  &  -iJ  &  0  & \lambda_E & 0\\
  0 & -iJ \sqrt{2} & 0  &  -iJ \sqrt{2}  &  iJ  & 0   & -iJ   & 0   &  0  &   \lambda_E \\
  \label{matrix_without_matter}
\end{bmatrix}}
\]
 \caption{Transformed Hamitonian evaluated over the transformed gauge invariant states.} %We can observe that it is similar to the one obtained in \ref{Matrix_with_matter}.}
  \label{Matrix_without_matter}
\end{figure}
